# Supplementary material for: Single-Qubit Gates Beyond the Rotating-Wave Approximation for Strongly Anharmonic Low-Frequency Qubits
Source: arXiv:2503.08238 source file (2025-03-11)
Supplement: Supplementary file 1 [file appendix_sw_1.tex]

\section{Schrieffer-Wolff transformation \label{app:sw}}
In this appendix, we detail the time-dependent Schrieffer-Wolff transformation applied to equation \ref{eq:drive_hamiltonian}. We split the Hamiltonian in an unperturbed part $H_0(t)$ and perturbation term $V(t)$:

\begin{equation}
\begin{split}
    H_0(t) &= \sum_{j \geq 1} \omega_j \ket{j}\bra{j} + \mathcal{D}(t) \Big(\ket{0}\bra{1}+\ket{1}\bra{0} \Big) \\
    V(t) &= \mathcal{D}(t)\sum_{j \geq 0, \; 0 \leq k < j, \; j,k \neq 0,1} \eta_{j-k,j} \Big(\ket{j}\bra{j-k} + \ket{j-k}\bra{j}\Big)
\end{split}
\end{equation}

We recall that we normalize the energies and drive strengths such that $\omega_0=0$ and $\eta_{01}=1$. Our objective is to perform a Schrieffer-Wolff transformation that cancels the perturbation term $V(t)$ up to first order. The first step is to diagonalize $H_0(t)=P(t)D(t)P^\dagger(t)$. The eigenvalues and eigenvectors of $H_0(t)$ are given by:

\begin{equation}
\begin{split}
    \lambda_0(t) = \frac{\omega_1}{2}-\frac{\sqrt{\omega_1^2+4\mathcal{D}(t)}}{2},& \quad \ket{\lambda_0(t)} = -\cos(\frac{\gamma(t)}{2})\ket{0} + \sin(\frac{\gamma(t)}{2})\ket{1}\\
    \lambda_1(t) = \frac{\omega_1}{2}+\frac{\sqrt{\omega_1^2+4\mathcal{D}(t)}}{2},& \quad \ket{\lambda_1(t)} = \sin(\frac{\gamma(t)}{2})\ket{0} + \cos(\frac{\gamma(t)}{2})\ket{1}\\
    \lambda_2 = \omega_2,& \quad \ket{\lambda_2} = \ket{2} \\
    \lambda_3 = \omega_3,& \quad \ket{\lambda_3} = \ket{3} 
\end{split}
\end{equation}

\noindent Such that $P(t)=\big[\ket{\lambda_0(t)},\ket{\lambda_1(t)},\ket{\lambda_2},\ket{\lambda_3}\big]$ and $D(t)=\text{diag}\big(\lambda_0(t),\lambda_1(t),\lambda_2,\lambda_3\big)$. Here, $\gamma(t) = \arctan(2\mathcal{D}(t)/\omega_1)$. Note that, since $H_0(t)$ is Hermitian, $P$ is guaranteed to be unitary. To diagonalize the Hamiltonian, we go into the rotating frame defined by $P^\dagger(t)$, but note that since $P(t=0)=P(t=t_g)=I$ we don't have to worry about actually applying these unitary transformations. Going into this frame gives:

\begin{equation}
\begin{split}
    \tilde{H}_0(t) &= D(t) \\
    \tilde{V}(t) &= \mathcal{D}(t)\sum_{j \geq 0, \; 0 \leq k < j, \; j,k \neq 0,1} \eta_{j-k,j} P^\dagger\Big(\ket{j}\bra{j-k} + \ket{j-k}\bra{j}\Big)P + \frac{\partial P^\dagger}{\partial t}
\end{split}
\end{equation}

This form is nice, because $\tilde{V}(t)$ is completely off-diagonal in the eigenbasis of $\tilde{H}_0(t)$. We will now derive the Schrieffer-Wolff transformation $S$, starting by writing the general form of the frame transformation:

\begin{equation}
\begin{split}
    H_\text{eff}(t) = & e^{iS(t)}\Big(\tilde{H}_0(t) + \tilde{V}(t)\Big)e^{-iS(t)} - \frac{\partial S(t)}{\partial t} \\
    = & \tilde{H}_0(t) + \tilde{V}(t) + i\Big[S(t),\tilde{H}_0(t)\Big] + i\Big[S(t),\tilde{V}(t)\Big] \\
    & - \frac{1}{2}\Big[S(t),\Big[S(t), \tilde{H}_0(t)\Big]\Big] - \frac{1}{2}\Big[S(t),\Big[S(t), \tilde{V}(t)\Big]\Big] - \frac{i}{6}\Big[S(t),\Big[S(t),\Big[S(t), \tilde{H}_0(t)\Big]\Big]\Big]
\end{split}
\end{equation}

\noindent To cancel the perturbation term up to first order, we require $\tilde{V}(t) + i\Big[S(t),\tilde{H}_0(t)\Big] - \frac{\partial S(t)}{\partial t} = 0$, to which the solution is:

\begin{equation}
    S_{ij}(t) = e^{-i(d_i-d_j)t}\int dt e^{i(d_i-d_j)t}\tilde{V}_{ij}(t)
\end{equation}

\noindent Which we can approximate using our favorite trick integration-by-parts as long as $\left|\frac{\partial^{k-1} \tilde{V}_{ij}(t)}{\partial t^{k-1}}\right| < |d_i-d_j|^{k}$ (with $k \geq 0$) by:

\begin{equation}
    S_{ij}(t) = \frac{1}{i}\frac{\tilde{V}_{ij}(t)}{d_i-d_j} + \frac{1}{(d_i-d_j)^2}\frac{\partial \tilde{V}_{ij}(t)}{\partial t}
\end{equation}

\noindent Plugging this back into equation ... gives the desired effective Hamiltonian:

\begin{equation}
\begin{split}
    H_\text{eff}(t) &= \frac{1}{2}\sum_k \tilde{V}_{ik}\tilde{V}_{kj}\left(\frac{1}{\lambda_i(t)-\lambda_k(t)} + \frac{1}{\lambda_k(t)-\lambda_j(t)}\right)
\end{split}
\end{equation}
