# Supplementary material for: Single-Qubit Gates Beyond the Rotating-Wave Approximation for Strongly Anharmonic Low-Frequency Qubits
Source: arXiv:2503.08238 source file (2025-03-11)
Supplement: Supplementary file 2 [file appendix_sw_2.tex]

\section{Schrieffer-Wolff Transformation 2.0}
Consider a Hamiltonian consisting of an unperturbed part $H_0$ and a perturbation $V$: $H(t) = H_0(t) + V(t)$. $H_0(t)$ is allowed to be time-dependent, but importantly we require the eigenvectors of $H_0$ to be time-independent, such that we can diagonalize $H_0(t)=PD(t)P^\dagger$. To derive the Schrieffer-Wolff transformation, we first transform the Hamiltonian to the frame $P^\dagger$:

\begin{equation}
\begin{split}
    \tilde{H}(t) &= P^\dagger H(t) P + i\dot{P}^\dagger P \\
    &= P^\dagger H_0(t) P + P^\dagger V(t) P \\
    &= D + V'(t)
\end{split}
\end{equation}

\noindent Crucially, since $P$ is time-independent, the term $i\dot{P}^\dagger P=0$. Also, note that this frame-transformation is not unique since the order of the eigenvectors in $P$ is ambiguous. We can now start the Schrieffer-Wolff transformation by transforming to into a second frame defined by $e^{S(t)}$:

\begin{equation}
\begin{split}
    \dbtilde{H}(t) &= e^S \tilde{H} e^{-S} + i\left(\frac{\partial}{\partial t}e^{S(t)}\right)e^{-S(t)} \\
    &= i\left(\frac{\partial}{\partial t}e^{S(t)}\right)e^{-S(t)} + D + V'(t) + [S(t),D] + [S(t),V'(t)] + \frac{1}{2}[S(t),[S(t),D]] + \dots 
\end{split}
\end{equation}

\noindent Here, an expansion in terms of $S(t)$ is justified if $S(t) \sim V'(t)$. To cancel the perturbation up to first order, we require $i\left(\frac{\partial}{\partial t}e^{S(t)}\right)e^{-S(t)} + V'(t) + [S(t),D]=0$. If $S(t)$ and $V(t)$ were time-independent, this is trivial to solve since $D$ is diagonal and one obtains: $S'_{ij} = V'_{ij}/(d_i-d_j)$. For time-dependent $S(t)$ and $V(t)$, we can only derive a straightforward solution if $[S(t),\dot{S}(t)]=0$, and we find:

\begin{equation}
    S_{ij}(t) = ie^{-i(d_i-d_j)t}\int_{-\infty}^t dt' e^{i(d_i-d_j)t}V'_{ij}(t) 
\end{equation}

Finally, we need to undo the two frame transformations in order to go back to the lab frame. In the context of this work, the Schrieffer-Wolff transformation is invoked to calculate some type of effective dynamics. Hence, we can try to engineer the Hamiltonian such that $S(t=t_0)=S(t_0+t_g)=0$, such that it intersects with the $P^\dagger$ frame at the start and end of the dynamics. Since $P^\dagger$ is unitary, it holds that $V'V'=P^\dagger V V P$. Hence, if $S(t)$ and $V(t)$ are time-independent, it is straightforward to derive the effective Hamiltonian in the lab frame up to second order in the perturbation:

\begin{equation}
    (H_\text{eff})_{ij} = (H_0)_{ij} + \frac{1}{2}\sum_kV_{ik}V_{kj}\left(\frac{1}{d_i-d_k} - \frac{1}{d_k-d_j}\right)
\end{equation}

Whether a straightforward solution exists for the time-dependent case depends on the time-complexity of $V'_{ij}(t)$, but an iterative solution can be computed using integration-by-parts if $\left|\frac{\partial^{k-1} \tilde{V}_{ij}(t)}{\partial t^{k-1}}\right| < |d_i-d_j|^{k}$ (with $k \geq 0$). For these solutions, going back to the lab frame is equally trivial since $P$ is time-independent.

If the eigenvectors of $H_0(t)$ are also time-dependent, an additional $i\dot{P}^\dagger P$ comes from the first frame transformation. With this term, we need to solve:

\begin{equation}
    \dot{S}(t) = iV'(t) + i[S(t),D(t) + i\dot{P}^\dagger(t) P(t)]
\end{equation}

\noindent Which is generally very challenging. Moreover, converting back to the lab frame after completing the frame transformations is no longer trivial as $\dot{V}'V' \neq P^\dagger \dot{V}V P$ since $P$ is now time-dependent.

Now, let's apply this knowledge on the problem of this work: modelling a strongly anharmonic system undergoing a drive as a two-level system. The Hamiltonian in an appropriate rotating frame is ($\hbar=1$):

\begin{equation}
\begin{split}
    &\tilde{H}(t) = \tilde{H}_0(t) + \tilde{V}(t) \\
    &\tilde{H}_0(t) = \sum_{1 \leq j \leq 3} (\omega_j-j\omega_d)\ket{j}\bra{j} + A_x(t)\sigma_x^{01} + A_y(t)\sigma_y^{01} \\
    &\tilde{V}(t) = \sum_{q \in \{x,y\}} \sum_{r \in \{12,23,03\}} \eta_r A^r_q(t) \sigma_q^r
\end{split}
\end{equation}

\noindent Here, $\sigma_x^{jk}=\ket{k}\bra{j}+\ket{j}\bra{k}$ and $\sigma_y^{jk}=i\ket{k}\bra{j}-i\ket{j}\bra{k}$ are the Pauli-$x$ and Pauli-$y$ operators acting on the transition $j \leftrightarrow k$. Furthermore, $A_q^{12}(t)=A_q^{23}(t)=A_q(t)$ and:

\begin{equation}
\begin{split}
    & A_x^{03}(t) = A_x(t)\cos(2\omega_dt+2\phi) - A_y(t)\sin(2\omega_dt+2\phi) \\
    & A_y^{03}(t) = A_y(t)\sin(2\omega_dt+2\phi) + A_x(t)\sin(2\omega_dt+2\phi)
\end{split}
\end{equation}

Notably, $V_{03}$ differs fundamentally in time-complexity from $V_{01}$, $V_{12}$ and $V_{23}$ and does not contain any stationary terms in this rotating frame. In the following, we set the rotation angle $\theta=0$ such that $A_x(t)$ and $A_y(t)$ correspond to $A_I(t)$ and $A_Q(t)$ in equation \ref{eq:hamiltonian-terms}. To derive an effective Hamiltonian for the qubit subspace, we would like to set-up a Schrieffer-Wolff transformation with $H_0(t)$ as the unperturbed Hamiltonian, and $V(t)$ as the perturbation. However, even if we would drive on resonance, the eigenvectors of $H_0(t)$ are time-dependent, complicating the Schrieffer-Wolff transformation as described above.

Motivated by the theory developed in this work, we assume that there exists a set of pulse parameters such that the oscillating non-RWA terms in $\tilde{H}_0$ are cancelled in the time evolution on the interval $t \in [t_0,t_0+N_ct_c]$, i.e.:

\begin{equation}
    \exists \; \hat{\tilde{H}}(t,\hat{\mathcal{P}}) \; : \; \int_{t_0}^{t_0+N_ct_c}dt \hat{\tilde{H}}(t,\hat{\mathcal{P}}) =  \int_{t_0}^{t_0+N_ct_c}dt \tilde{H}(t,\mathcal{P})
\end{equation}

\noindent Where, similar to the main text, the Hamiltonians depend explicitly on the pulse parameters to highlight that they are different for $\tilde{H}(t)$ and $\hat{\tilde{H}}(t)$. Here, we would like $\hat{\tilde{H}}$ to take the following form:

\begin{equation}
\begin{split}
    &\hat{\tilde{H}}(t) = \hat{\tilde{H}}_0(t) + \hat{\tilde{V}}(t) \\
    &\tilde{H}_0(t) = \sum_{1 \leq j \leq 3} (\omega_j-j\omega_d)\ket{j}\bra{j} + \mathcal{E}_x(t)\sigma_x^{01} + \mathcal{E}_y(t)\sigma_y^{01} \\
    &\tilde{H}
\end{split}
\end{equation}

\noindent Where $\mathcal{E}_x(t)=\text{Re}(\mathcal{E}(t))$ and $\mathcal{E}_y(t)=\text{Im}(\mathcal{E}(t))$.
